# Supplementary material for: Improved Submodular Secretary Problem with Shortlists
Source: arXiv:2010.01901 source file (2021-02-19)
Supplement: Supplementary file 2 [file Suppanlysis.tex]

\toRemove{
\newcommand{\settinga}{\mbox{$k \ge \alpha\beta$}, \settingb}
\newcommand{\settingb}{\mbox{$\beta\ge \frac{8}{(\delta')^2}$}, $\alpha\ge 8\beta^2 \log(1/\delta')$}
}

\toRemove{

In this section we show that for any $\epsilon \in (0,1)$, Algorithm \ref{alg:tmp} with an appropriate choice of constants $\alpha, \beta$, achieves the competitive ratio claimed in Theorem \ref{opttheorem} for the \nameOfProblemMatroidSL.  

%Recall the following notation defined in the previous section.  For any collection of sets $V_1, \ldots, V_\ell$, we use $V_{1,\ldots, \ell}$ to denote $V_1 \cup \cdots \cup V_\ell$. Also, recall that for any item $i$ and set $V $, we denote $\Delta_f(i|V):=f(V\cup \{i\})- f(V)$.
\toRemove{
\paragraph{Proof overview.} The proof is divided into two parts. We first  show a lower bound on the ratio $\Ex[f(S_{1,\cdots,W})]/{\OPT}$ in Proposition~\ref{prop:first}, where $S_w$ is the subset of items as defined in \eqref{eq:Sw} for every window $w$. Later in Proposition~\ref{prop:online}, we use the said  bound to derive a lower bound on the ratio $\Ex[f(A^*)]/\OPT$, where $A^*=A\cap (S_{1,\cdots, W})$ is the subset of shortlist returned by Algorithm~\ref{alg:main}. %This will complete the proof of Theorem \ref{opttheorem}.

Specifically, in Proposition \ref{prop:first}, we provide settings of parameters $\alpha, \beta$ such that of $\Ex[f(S_{1,\cdots, W})] \ge \left(1-\frac{1}{e}-\frac{\epsilon}{2} - O(\frac{1}{k})\right)\OPT$.  A central idea in the proof of this result is to show that for every window $w$, given $R_{1,\ldots, w-1}$,  the items tracked from the previous windows, any of the $k$ items from the optimal set $S^*$ (if the independent set has less than $k$ items extend it by adding some dummy items) has at least $\frac{\alpha}{k}$ probability to appear either in window $w$, or among the tracked items $R_{1,\ldots, w-1}$. Further, the items from $S^*$ that appear in window $w$, appear  independently, and in a uniformly at random slot in this window. (See Lemma \ref{lem:pijBound}.)  This observation allows us to show that, in each window, there exists a subsequence $\tilde \tau_w$ of close to $\alpha$ slots, such that the greedy sequence of items $\gamma(\tilde \tau_w)$ will be almost ``as good as" a randomly chosen sequence of $\alpha$ items from $S^*$. More precisely, denoting $\gamma(\tilde \tau_s)=(i_1,\ldots, i_t)$, in Lemma \ref{lem:asGoodas}, for all $j=1,\ldots, t$, we lower bound the increment in function value $f(\cdots)$ on adding $i_j$ over the items in $S_{1, \ldots, w-1} \cup i_{1,\ldots, j-1}$ as:
{\small $$\Ex[\Delta_f(i_j|S_{1,\ldots, w-1} \cup \{i_1, \ldots, i_{j-1}\})|T_{1,\ldots, w-1}, i_1, \ldots, i_{j-1}] \ge \frac{1}{k}\left((1-\frac{\alpha}{k})f(S^*)-f(S_{1,\ldots, w-1} \cup \{i_1, \ldots, i_{j-1}\})\right)\ . $$}
We then deduce (using standard techniques for the analysis of greedy algorithm for submodular functions) that 
{\small $$\Ex[\left(1-\frac{\alpha}{k}\right) f(S^*) - f(S_{1,\ldots, w-1}\cup \gamma(\tilde \tau_w)) | S_{1,\ldots, w-1}] \le e^{-t/k} \left(\left(1-\frac{\alpha}{k}\right) f(S^*)-f(S_{1,\ldots, w-1})\right)\ .$$}
%Further, we show that $t$ is close to $\alpha$ with high probability (refer to Lemma \ref{lem:}). 
Now, since the length $t$ of $\tilde \tau_w$ is close to $\alpha$ (as we show in Lemma \ref{lem:lengthtau}) and since  $S_w=\gamma(\tau^*)$ with $\tau^*$ defined as the ``best"  subsequence of length $\alpha$ (refer to definition of $\tau^*$ in \eqref{eq:taustar}), we can show that a similar inequality holds for {\small $S_w=\gamma(\tau^*)$, i.e.,
$$\left(1-\frac{\alpha}{k}\right) f(S^*) - \Ex[f(S_{1,\ldots, w-1}\cup S_w)|S_{1,\ldots, w-1}] \le e^{-\alpha/k} \left(1-\delta'\right)\left(\left(1-\frac{\alpha}{k}\right) f(S^*)-f(S_{1,\ldots, w-1})\right)\ ,$$}
where $\delta'\in (0,1)$ depends on the setting of $\alpha, \beta$. (See   Lemma~\ref{lem:Sw}.)  Then repeatedly applying this inequality for $w=1, \ldots, k/\alpha$, and setting $\delta, \alpha, \beta$ appropriately in terms of $\epsilon$, we can obtain $\Ex[f(S_{1,\ldots, W})] \ge \left(1-\frac{1}{e^2} - \frac{\epsilon}{2} -\frac{1}{k}\right) f(S^*)$, completing  the proof of Proposition \ref{prop:first}.

However, a remaining difficulty is that while the algorithm keeps a track of the set $S_w$ for every window $w$, it may not have been able to add all the items in $S_w$ to the shortlist $A$ during the online processing of the inputs in that window. In the proof of Proposition \ref{prop:online}, we show that in fact the algorithm will add most of the items in $\cup_w S_w$ to the short list. More precisely, we show that given that an item $i$ is in $S_w$, it will be in shortlist $A$ with probability $1-\delta$, where $\delta$ is the parameter used while calling Algorithm \ref{alg:SIIImax} in Algorithm \ref{alg:main}. Therefore, using properties of submodular functions it follows  that with $\delta=\epsilon/2$, $\Ex[f(A^*)] = \Ex[f( S_{1,\cdots, W} \cap A)] \ge (1-\frac{\epsilon}{2})\Ex[f(S_{1,\cdots, W})]$ (see Proposition \ref{prop:online}). Combining this with the lower bound $\frac{\Ex[f(S_{1,\cdots, W})]}{\OPT} \ge (1-\frac{1}{e^2}-\frac{\epsilon}{2} - O(\frac{1}{k}))$ mentioned earlier, we complete the proof of competitive ratio bound stated in Theorem \ref{opttheorem}.
%The set $A^*$ returned by Algorithm \ref{alg:tmp} is $\cup_w (S_w\cap H_w)$. we complete the proof of Theorem \ref{opttheorem} by showing that each item in $S_w$ will appear in $H_w$ with a high enough probability,

}

}

%\subsection{Bounding $\Ex[f( S_{1,\cdots, W})]/\OPT$}
 
%%%%%%%%%%%%%%%%%%%%
%\input{newProof.tex}
%\input{twocol/Supp/newProof}
\toRemove{
First, we use the observations from the previous sections to show the existence of a random subsequence of slots $\tilde \tau_w$ of window $w$ such that we can lower bound $f((S_{1,\ldots, w-1}\cup \gamma(\tilde \tau_w))\setminus \zeta(\tilde \tau_w))- f(S_{1,\ldots, w-1})$ in terms of $\OPT -f(S_{1,\ldots, w-1})$. This will be used to lower bound  increment %$\Delta_f(S_w|S_{1,\ldots, w-1}) = 
$f(S_{1,\ldots, w-1}\cup \gamma(\tau^*)\setminus \zeta(\tau^*)) -f(S_{1,\ldots, w-1})$ in every window.

%For any item $i\in S^*$, window $w \in \{1,\ldots, W\}$, and slot $s$ in window $w$, define
%\begin{equation}
%\label{eq:pijBound}
%p_{is}:=\mathbb{P}(i \in s \cup Supp(T) | T_{1,\ldots, w-1}=T).
%\end{equation}

\begin{definition}[$Z_s$ and $\tilde \gamma_w$]
\label{def:tauw}
Create sets of items $Z_s, \forall s\in w$  as follows: for every slot $s$, add every item from $i\in S^*\cap s$ independently with probability $\frac{1}{k \beta p_{is}}$ to $Z_s$. Then, for every item $i\in S^*\cap T$, with probability $\alpha/k$, add $i$ to $Z_s$ for a randomly chosen slot $s$ in $w$. Define subsequence $\tilde \tau_w$ as the sequence of 
slots with $Z_s\ne \emptyset$. 
\end{definition}
}

\toRemove{
Similar to~\cite{us}, we have the following property for $Z_s$:
\begin{lemma}
\label{lem:Zs}
Given any $T_{1,\ldots, w-1}=T$, for any slot $s$ in window $w$, all $i, i' \in S^*, i\ne i'$ will appear in $Z_s$ independently with probability $\frac{1}{k\beta}$. Also, given $T$, for every $i \in S^*$, the probability to appear in $Z_s$ is equal for all slots $s$ in window $w$. Further, each $i\in S^*$ occurs in  $Z_s$ of at most one slot $s$.
\end{lemma}
}

\mcomment{
In the following lemmas suppose the sequence $\tilde \tau_w=(s_1, \ldots, s_t)$, and $Z_{s_1} \cup \ldots \cup Z_{s_{j-1}}$ defined as in Definition \ref{def:tauw}, let $\gamma(\tilde \tau_s)=(i_1,\ldots, i_t)$, with $\gamma(\cdot)$ as defined in \eqref{eq:gamma}.
}

\toRemove{
\begin{lemma}
For all $i, i' \in S^*\backslash \{Z_{s_1} \cup \ldots \cup Z_{s_{j-1}}\}$,
\begin{align*} 
\label{eq:pk}
&\Pr(i\in Z_{s_j}| Z_{s_1}, \ldots , Z_{s_{j-1}}, T_{1,\cdots, w-1})
= \Pr(i'\in Z_{s_j}| Z_{s_1}  \ldots  Z_{s_{j-1}},T_{1,\cdots, w-1})  
\ge \frac{1}{k} \ .
\end{align*}
\end{lemma}
}

\mcomment{
\textbf{Proof of Lemma~\ref{lemma:zs}}.
\begin{proof}
The proof is similar to eq.~(10) in Lemma 11 of~\cite{us}, and it is based on Lemma \ref{lem:Zs},
\end{proof}
}

\toRemove{
\begin{lemma}
We can show that for all $i, i' \in S^*\backslash \{Z_{s_1} \cup \ldots \cup Z_{s_{j-1}}\}$,
\begin{equation} 
\label{eq:pk}
\Pr(i\in Z_{s_j}| Z_{s_1} \cup \ldots \cup Z_{s_{j-1}}) = \Pr(i'\in Z_{s_j}| Z_{s_1} \cup \ldots \cup Z_{s_{j-1}})  \ge \frac{1}{k} \ .
\end{equation}
\end{lemma}
\begin{proof}
The proof is similar to Lemma 12 in~\cite{us}, and it is based on Lemma \ref{lem:Zs},
\end{proof}
}

\mcomment{
In the following lemma we lower bound the marginal gain of a randomly picked element of optimal solution in slot $s_j$ with respect to previously selected items.
}

%\subsection{Proof of lemma 7}

\toRemove{
\begin{lemma} 
\label{lem:asGoodas}
(proof of lemma 7)
Suppose the sequence $\tilde \tau_w=(s_1, \ldots, s_t)$ defined as in Definition \ref{def:tauw}, let $\gamma(\tilde \tau_s)=(i_1,\ldots, i_t)$, with $\gamma(\cdot)$ as defined in \eqref{eq:gamma}. Then, for all $j=1,\ldots, t$, 
%given $a\in S^*\cap Z_{s_j}$.

{\small \begin{eqnarray*}
\Ex[\Delta_f(a|S_{1,\ldots, w-1} \cup \{i_1, \ldots, i_{j-1}\}\setminus\{c_1,\cdots, c_{j-1}\})|T_{1,\ldots, w-1}, i_{1,\ldots, j-1}, a\in S^*\cap Z_{s_j}]\\
 \ge \frac{1}{k}\left((1-\frac{\alpha}{k})f(S^*)-f(S_{1,\ldots, w-1} \cup \{i_1, \ldots, i_{j-1}\}\setminus\{c_1,\cdots,c_{j-1}\})\right)\
\end{eqnarray*}}
\end{lemma}
}

%\subsection

\mcomment{
\textbf{Proof of Lemma~\ref{lem:asGoodas}}
\begin{proof}
We can lower bound the increment assuming $a$ is randomly picked item from $Z_{s_j}\cap S^*$:
\begin{eqnarray*} 
& & \Ex[\Delta_f(a,S(w-1,\tilde{\tau}_w,j-1)) |T_{1,\ldots, w-1}=T, i_1, \ldots, i_{j-1},a\in S^*\cap Z_{s_j}] \\
& \ge & \frac{1}{k} \Ex[\sum_{a\in S^*\backslash \{Z_1,\ldots Z_{s_{j-1}}\}} \Ex[\Delta_f(a,S(w-1,\tilde{\tau}_w,j-1))|T, i_1, \ldots, i_{j-1}]] \\
%(\text{using  Lemma~\ref{marginalsum}, monotonicity of $f$} ) 
& \ge & \frac{1}{k} \Ex[ (f(S^*\backslash  \{Z_1,\ldots Z_{s_{j-1}}\})-f(S(w-1,\tilde{\tau}_w,j-1))) | T]\\
%(\text{using  monotonicity of }f)
& \ge & \frac{1}{k}  \Ex[(f(S^*\backslash  \cup_{s'\in w} Z_{s'})-f(S(w-1,\tilde{\tau}_w,j-1))| T]\\
& \geq & \frac{1}{k} ((1-\frac{\alpha}{k})f(S^*) -f(S(w-1,\tilde{\tau}_w, j-1)).
\end{eqnarray*}
%Here, we used the submodularity of $f$ and 
The last inequality uses 
Lemma \ref{sample} for submodular function $f$,
and the observation from Lemma \ref{lem:Zs} that given $T$, every $i\in S^*$ appears in $\cup_{s'\in w} Z_{s'}$ independently with probability $\alpha/k$, so that every $i\in S^*$ appears in $S^*\backslash\cup_{s'\in w} Z_{s'}$ independently with probability $1-\frac{\alpha}{k}$; %along with Lemma \ref{sample} for submodular function $f$. 
%so that $\Ex[|\cup_{s'\in w} Z_{s'}|] \le {\alpha}$.
\end{proof}
}

%\subsection

\mcomment{
\textbf{Proof of Lemma~\ref{replaced}}
\begin{proof}
%It follows from Brualdi lemma and lemma~\ref{sample}.
Since $\pi$ is a bijection from $S^*$ to $S'$, from Brualdi's lemma (lemma~\ref{lem:Brualdi}), there is an onto mapping $\pi'$ from $S^*$ %$OPT$ 
 to $S(w-1,\tilde{\tau}_w,j-1)\cup \{\emptyset\}$ 
such that 
$S(w-1,\tilde{\tau}_w,j-1)- \pi'(a) +a \in \mathcal{I}$, for all $a \in S^*$. Further, $\pi'(a)=\pi(a)$ if $\pi(a)\in  S(w-1,\tilde{\tau}_w,j-1)$ and $\pi'(a)=\emptyset$ otherwise.
%Note that $\pi$ maps some $a \in S^*$, to the empty set, i.e., we set $\pi(a)=\emptyset$.
Recall the definition of $Z_{s_j}$.
%Recall the definition $Z_{s_j}$ defined in the last paper.
%\begin{definition}[$Z_s$ and $\tilde \gamma_w$]
%\label{def:tauw}
%Create sets of items $Z_s, \forall s\in w$  as follows: for every slot $s$, add every item from $i\in S^*\cap s$ independently with probability $\frac{1}{k \beta p_{is}}$ to $Z_s$. Then, for every item $i\in S^*\cap T$, with probability $\alpha/k$, add $i$ to $Z_s$ for a randomly chosen slot $s$ in $w$.
%Define subsequence $\tilde \tau_w$ as the sequence of slots with $Z_s\ne \phi$. 
%Suppose $|Z_{s_j}|=1$ and $S^*\cap Z_{s_j}=a$.
Suppose $a$ is a randomly picked item from $S^*\cap Z_{s_j}$.
%(in terms of notation defined in last paper $Z_{s_j}=1$)
Note that from Lemma~\ref{lem:Zs}, conditioned on $T_{1,\cdots, w-1}$ and $i_1,\cdots,i_{j-1}$, the element $a$ can be equally any element of %$S^*$ 
%$S^*\backslash  \{Z_1,\ldots Z_{s_{j-1}}\}$
$S^*\backslash  \{i_1,\ldots i_{{j-1}}\}$
with probability
%at least
$1/(k-\alpha)$.
%$1/k$.
Therefore, $\pi'(a)$ would be any of $S(w-1,\tilde{\tau},j-1)$ with probability at most %$1/k$ 
$1/(k-\alpha)$ 
%(note that $|S_{1,\cdots, w-1}\cup \{i_1, \cdots, i_{j-1}\}\setminus \{c_1,\cdots, c_{j-1}\}| < k$, thus sometimes $\pi(a)$ might not be defined).
(since $\pi'$ might map some elements of $S^*$ to the empty set).
Now based on the definition of $\pi$ and lemma~\ref{sample} we have:
{\small \begin{eqnarray*}
\Ex[f(S(w-1,\tilde{\tau}_w,j-1)\setminus\{\pi(a)\})|T_{1,\ldots, w-1}, i_{1,\ldots, j-1}, a\in S^*\cap Z_{s_j}]
 \ge (1-\frac{1}{k-\alpha})f(S(w-1,\tilde{\tau}_w,j-1)\}).\
\end{eqnarray*}}
\end{proof}
}

\toRemove{
\begin{lemma}\label{replaced}
%At the end of window $w$, 
Suppose the sequence $\tilde \tau_w=(s_1, \ldots, s_t)$ defined as in Definition \ref{def:tauw}, let $\gamma(\tilde \tau_s)=(i_1,\ldots, i_t)$, with $\gamma(\cdot)$ as defined in \eqref{eq:gamma}. 
Moreover, let $S'$ be the extension of $S_{1,\cdots, w-1}\cup \{i_1, \cdots, i_{j-1}\}\setminus \{c_1,\cdots, c_{j-1}\}$ to an independent set in $\mathcal{M}$, and $\pi$ be the bijection from Brualdi lemma (refer to Lemma~\ref{lem:Brualdi}) from $S^*$ to $S'$.
Then, for all $j=1,\ldots, t$, \\
{\small \begin{eqnarray*}
\Ex[f(S_{1,\ldots, w-1} \cup \{i_1, \ldots, i_{j-1}\}\setminus\{c_1,\cdots, c_{j-1},\pi(a)\})|T_{1,\ldots, w-1}, i_{1,\ldots, j-1}, a\in S^*\cap Z_{s_j}]\\
 \ge (1-\frac{1}{k-\alpha})f(S_{1,\ldots, w-1} \cup \{i_1, \ldots, i_{j-1}\}\setminus\{c_1,\cdots,c_{j-1}\})\
\end{eqnarray*}}
\toRemove{
{\small \begin{eqnarray*}
\Ex[\Delta_f(a|S_{1,\ldots, w-1} \cup \{i_1, \ldots, i_{j-1}\}\setminus\{c_1,\cdots, c_{j-1},\pi(a)\})|T_{1,\ldots, w-1}, i_{1,\ldots, j-1}, a\in S^*\cap Z_{s_j}]\\
 \ge (1-\frac{1}{k})f(S^*)-f(S_{1,\ldots, w-1} \cup \{i_1, \ldots, i_{j-1}\}\setminus\{c_1,\cdots,c_{j-1}\}\
\end{eqnarray*}}
}
%$\mathbb{E}[f(S_{1,\cdots, w-1}\cup \{i_1, \ldots, i_{j-1}\} \setminus \{c_1,\cdots, c_{j-1}, \pi(a)\} ] \ge (1-\frac{1}{k}) f(S_{1,\cdots, w-1}\cup \{i_1, \ldots, i_{j-1}\} \setminus \{c_1, \cdots, c_{j-1}\} )$$
\end{lemma}
\begin{proof}
%It follows from Brualdi lemma and lemma~\ref{sample}.
Since $\pi$ is a bijection from $S^*$ to $S'$, from Brualdi's lemma (lemma~\ref{lem:Brualdi}), there is an onto mapping $\pi'$ from $S^*$ %$OPT$ 
 to $S_{1,\cdots, w-1}\cup \{i_1, \cdots, i_{j-1}\}\setminus \{c_1,\cdots, c_{j-1}\}\cup \{\emptyset\}$ 
such that %$S_{1,\cdots, w-1}\cup \{i_1, \ldots, i_{j-1}\} - \pi(a) +a \in M$ for all $a \in S^*$.
$S_{1,\cdots, w-1}\cup \{i_1, \cdots, i_{j-1}\}\setminus \{c_1,\cdots, c_{j-1}\}- \pi'(a) +a \in M$, for all $a \in S^*$. Further, $\pi'(a)=\pi(a)$ if $\pi(a)\in  S_{1,\cdots, w-1}\cup \{i_1, \cdots, i_{j-1}\}\setminus \{c_1,\cdots, c_{j-1}\}$ and $\pi'(a)=\emptyset$ otherwise.

%Note that $\pi$ maps some $a \in S^*$, to the empty set, i.e., we set $\pi(a)=\emptyset$.

Recall the definition of $Z_{s_j}$.
%Recall the definition $Z_{s_j}$ defined in the last paper.
%\begin{definition}[$Z_s$ and $\tilde \gamma_w$]
%\label{def:tauw}
%Create sets of items $Z_s, \forall s\in w$  as follows: for every slot $s$, add every item from $i\in S^*\cap s$ independently with probability $\frac{1}{k \beta p_{is}}$ to $Z_s$. Then, for every item $i\in S^*\cap T$, with probability $\alpha/k$, add $i$ to $Z_s$ for a randomly chosen slot $s$ in $w$. 
%Define subsequence $\tilde \tau_w$ as the sequence of slots with $Z_s\ne \phi$. 
%Suppose $|Z_{s_j}|=1$ and $S^*\cap Z_{s_j}=a$.
Suppose $a$ is a randomly picked item from $S^*\cap Z_{s_j}$.
%(in terms of notation defined in last paper $Z_{s_j}=1$)
Note that from Lemma~\ref{lem:Zs}, conditioned on $T_{1,\cdots, w-1}$, the element $a$ can be equally any element of %$S^*$ 
$S^*\backslash  \{Z_1,\ldots Z_{s_{j-1}}\}$
with probability at least $1/(k-\alpha)$.
Therefore, $\pi'(a)$ would be any of $S_{1,\cdots, w-1}\cup \{i_1, \cdots, i_{j-1}\}\setminus \{c_1,\cdots, c_{j-1}\}$ with probability at most $1/(k-\alpha)$ %(note that $|S_{1,\cdots, w-1}\cup \{i_1, \cdots, i_{j-1}\}\setminus \{c_1,\cdots, c_{j-1}\}| < k$, thus sometimes $\pi(a)$ might not be defined).
(since $\pi'$ might map some elements of $S^*$ to the empty set).
Now based on the definition of $\pi$ and lemma~\ref{sample} we have:

{\small \begin{eqnarray*}
\Ex_a[f(S_{1,\ldots, w-1} \cup \{i_1, \ldots, i_{j-1}\}\setminus\{c_1,\cdots, c_{j-1},\pi(a)\})|T_{1,\ldots, w-1}, i_{1,\ldots, j-1}, a\in S^*\cap Z_{s_j}]\\
 \ge (1-\frac{1}{k-\alpha})f(S_{1,\ldots, w-1} \cup \{i_1, \ldots, i_{j-1}\}\setminus\{c_1,\cdots,c_{j-1}\})\
\end{eqnarray*}}

\toRemove{
{\small \begin{eqnarray*}
\Ex_a[\Delta_f(a|S_{1,\ldots, w-1} \cup \{i_1, \ldots, i_{j-1}\}\setminus\{c_1,\cdots, c_{j-1},\pi(a)\})|T_{1,\ldots, w-1}, i_{1,\ldots, j-1}, a\in S^*\cap Z_{s_j}]\\
 \ge (1-\frac{1}{k})f(S^*)-f(S_{1,\ldots, w-1} \cup \{i_1, \ldots, i_{j-1}\}\setminus\{c_1,\cdots,c_{j-1}\}\
\end{eqnarray*}}
}
%$$ \mathbb{E}[f(S_{1,\cdots, w-1} \cup \{i_1, \cdots, i_{j-1}\} \setminus \{c_1, \cdots, c_{j-1} , \pi(a)\} )] \ge (1-1/k) f(S_{1,\cdots, w-1} \cup \{i_1, \cdots, i_{j-1}\} \setminus \{c_1, \cdots, c_{j-1}\} ) $$

%Note that $g(e,S) \ge \Delta_f(e|S) $.
%Note that $g(e,S) \ge f(S+e-\pi(e) )  -f(S)$.
%Therefore 
%Note that $\bar{S}_w:=\zeta(\tau^*)=\{c_1, \cdots, c_{\ell}\}$.
\end{proof}

\begin{lemma}\label{exg}
%We can show that:
%\begin{align}\label{recursion}
Suppose function $g$ is as defined in equation~\ref{eq:g}.
For the sequence $\tilde \tau_w=(s_1, \ldots, s_t)$, and $\gamma(\tilde \tau_s)=(i_1,\ldots, i_t)$. Then, for all $j=1,\ldots, t$, \\
{\small \begin{eqnarray*}
\Ex[g(i_j,S_{1,\ldots, w-1} \cup \{i_1, \ldots, i_{j-1}\}\setminus\{c_1,\cdots, c_{j-1}\})|T_{1,\ldots, w-1}, i_{1,\ldots, j-1}]\\
 \ge 
 %(1-\frac{1}{k-\alpha})
 \frac{1}{k}
 \left(
 (1-\frac{\alpha}{k-\alpha})f(S^*)-
 2f(S_{1,\ldots, w-1} \cup \{i_1, \ldots, i_{j-1}\}\setminus\{c_1,\cdots,c_{j-1}\})\right)\
\end{eqnarray*}}

\toRemove{
$$ 
\Ex[g(i_j,{S}_{1,\ldots, w-1} \cup \{i_1,\cdots,i_{j-1}\}\setminus \{c_1,\cdots, c_{j-1}\})|T_{1,\cdots, w-1},i_{1,\cdots, j-1}]
$$
$$
\ge
{ \frac{1}{k}\left((1-\frac{\alpha}{k})f(S^*)-2f({S}_{1,\ldots, w-1} \cup \{i_1,\cdots,i_{j-1}\}\setminus \{c_1,\cdots, c_{j-1}\})\right)\ . }
$$  
}
%\end{align}
\end{lemma}

\begin{proof}
In the algorithm~\ref{alg:main}, at the end of window $w$, we set %$S_{1,\cdots, w-1} = {S}_{1,\cdots, w-1} \setminus \bar{S}_w$.
$S_{1,\cdots, w} = S_{1,\cdots, w-1}\cup S_w \setminus \bar{S}_w$.
Suppose $a\in s_j\cap S^*$. 
Moreover, let $S'$ be the extension of $S_{1,\cdots, w-1}\cup \{i_1, \cdots, i_{j-1}\}\setminus \{c_1,\cdots, c_{j-1}\}$ to an independent set in $\mathcal{M}$, and $\pi$ be the bijection from Brualdi lemma (refer to Lemma~\ref{lem:Brualdi}) from $S^*$ to $S'$.
Thus the expected value of the function $g$ on the element selected by the algorithm in slot $s_j$ (the element with maximum $g$ in the slot $s_j$) would be
\begin{eqnarray*}
%\begin{align}
%g(i_j,{S}_{1,\ldots, w-1} \cup \{i_1,\cdots,i_{j-1}\}\setminus \{c_1,\cdots, c_{j-1}\})
%= 
&\Ex[f({S}_{1,\ldots, w-1} \cup \{i_1, \ldots, i_{j}\} \setminus \{c_1,\cdots, c_j \}|T_{1,\ldots, w-1}, i_{1,\ldots, j-1}]  %- f(S_{1,\cdots, w-1}\cup \{i_1, \ldots, i_{j-1}\} \setminus \{c_1,\cdots, c_{j-1}\}) 
\\\ge&
\Ex[f({S}_{1,\ldots, w-1} \cup \{i_1, \ldots, i_{j-1}, a\} \setminus \{c_1,\cdots, c_{j-1}, \pi(a) \} |T_{1,\ldots, w-1}, i_{1,\ldots, j-1}, a\in S^*\cap Z_{s_j}] %- f(S_{1,\cdots, w-1}\cup \{i_1, \ldots, i_{j-1}\} \setminus \{c_1,\cdots, c_{j-1} \}) 
\\\ge&
%f({S}_{1,\ldots, w-1} \cup \{i_1, \ldots, i_{j-1}, a\} \setminus \{c_1,\cdots, c_{j-1}, \pi(a) \} )-
\Ex[f({S}_{1,\ldots, w-1} \cup \{i_1, \ldots, i_{j-1}\} \setminus \{c_1,\cdots, c_{j-1}, \pi(a) \} )|T_{1,\ldots, w-1}, i_{1,\ldots, j-1}, a\in S^*\cap Z_{s_j}]
\\&+\Ex[\Delta_f(a|S_{1,\cdots,w-1}\cup\{i_1,\cdots,i_{j-1}\}\setminus \{c_1,\cdots, c_{j-1},\pi(a)\} )|T_{1,\ldots, w-1}, i_{1,\ldots, j-1}, a\in S^*\cap Z_{s_j}] \\
\ge&
\Ex[f({S}_{1,\ldots, w-1} \cup \{i_1, \ldots, i_{j-1}\} \setminus \{c_1,\cdots, c_{j-1}, \pi(a) \} )|T_{1,\ldots, w-1}, i_{1,\ldots, j-1}, a\in S^*\cap Z_{s_j}]
\\&+\Ex[\Delta_f(a|S_{1,\cdots,w-1}\cup\{i_1,\cdots,i_{j-1}\}\setminus \{c_1,\cdots, c_{j-1}\} )|T_{1,\ldots, w-1}, i_{1,\ldots, j-1}, a\in S^*\cap Z_{s_j}]
%\end{align}
\end{eqnarray*}
The first inequality is from the definition of function $g$ as it is defined in equation~\ref{eq:g}. The last inequality from submoularity of $f$.
Now from the last inequality  and lemma~\ref{replaced} we have
\begin{align*}
&\Ex[f({S}_{1,\ldots, w-1} \cup \{i_1, \ldots, i_{j}\} \setminus \{c_1,\cdots, c_j \} |T_{1,\ldots, w-1}, i_{1,\ldots, j-1})]& \\ &\ge
%f({S}_{1,\ldots, w-1} \cup \{i_1, \ldots, i_{j-1}, a\} \setminus \{c_1,\cdots, c_{j-1}, \pi(a) \} )\ge 
(1-\frac{1}{k-\alpha} ) f(S_{1,\cdots, w-1}\cup \{i_1, \ldots, i_{j-1}\} \setminus \{c_1, \cdots, c_{j-1}\} )&\\
&+ \Ex[ \Delta_f(a|{S}_{1,\ldots, w-1} \cup \{i_1, \ldots, i_{j-1}\} \setminus\{c_1,\cdots, c_{j-1}\} \})||T_{1,\ldots, w-1}, i_{1,\ldots, j-1}, a\in S^*\cap Z_{s_j}] &
\end{align*}
Now from lemma~\ref{lem:asGoodas} and the above inequality we can show
\begin{align*}
&\Ex[f({S}_{1,\ldots, w-1} \cup \{i_1, \ldots, i_{j}\} \setminus \{c_1,\cdots, c_j \} |T_{1,\ldots, w-1}, i_{1,\ldots, j-1})]& \\  &\ge
%f({S}_{1,\ldots, w-1} \cup \{i_1, \ldots, i_{j-1}, a\} \setminus \{c_1,\cdots, c_{j-1}, \pi(a) \} )\ge 
(1-\frac{1}{k-\alpha} ) f(S_{1,\cdots, w-1}\cup \{i_1, \ldots, i_{j-1}\} \setminus \{c_1, \cdots, c_{j-1}\} )&\\
&+{ \frac{1}{k}\left((1-\frac{\alpha}{k})f(S^*)-f({S}_{1,\ldots, w-1} \cup \{i_1, \ldots, i_{j-1}\} \setminus\{c_1,\cdots, c_{j-1}\})\right)\ . }&
\end{align*}
Thus,
\begin{align}\label{recursion}
f({S}_{1,\ldots, w-1} \cup \{i_1, \ldots, i_{j}\} \setminus \{c_1,\cdots, c_j \} )  
%f({S}_{1,\ldots, w-1} \cup \{i_1, \ldots, i_{j-1}, a\} \setminus \{c_1,\cdots, c_{j-1}, \pi(a) \} )\ge 
- f(S_{1,\cdots, w-1}\cup \{i_1, \ldots, i_{j-1}\} \setminus \{c_1, \cdots, c_{j-1}\} )\\
\ge
{ \frac{1}{k}\left((1-\frac{\alpha}{k})f(S^*)-2f({S}_{1,\ldots, w-1} \cup \{i_1,\cdots,i_{j-1}\}\setminus \{c_1,\cdots, c_{j-1}\})\right)\ . }
\end{align}

\end{proof}

Using standard techniques for the analysis of greedy algorithm, the following corollary of the previous lemma can be derived, 

}

\mcomment{
\textbf{Proof of Lemma~\ref{exg}}
}

\toRemove{
\begin{lemma}\label{exg}
Suppose function $g$ is as defined in equation~\eqref{eq:g}, and $\rho:=\frac{k}{k-\alpha}$.
For all $j=1,\ldots, t$, \\
{\small \begin{eqnarray*}
&\Ex[g(i_j,S(w-1,\tilde{\tau}_w,j-1)) | T_{1,\cdots, w-1}, i_{1,\ldots, j-1}] \ge 
 %(1-\frac{1}{k-\alpha})
 \frac{1}{k}
 ((1-\frac{\alpha}{k})f(S^*)-
 2\rho f(S(w-1,\tilde{\tau}_w,j-1))).\
\end{eqnarray*}}
\toRemove{
{\small \begin{eqnarray*}
&\Ex[g(i_j,S_{1,\ldots, w-1} \cup \{i_1, \ldots, i_{j-1}\}\setminus\{c_1,\cdots, c_{j-1}\}) | T, i_{1,\ldots, j-1}]\\
 &\ge 
 %(1-\frac{1}{k-\alpha})
 \frac{1}{k}
 ((1-\frac{\alpha}{k-\alpha})f(S^*)-
 2f(S_{1,\ldots, w-1} \cup 
 \{i_1, \ldots,i_{j-1}\}\setminus\{c_1,\cdots,c_{j-1}\})).\
\end{eqnarray*}}
}
\toRemove{
$$ 
\Ex[g(i_j,{S}_{1,\ldots, w-1} \cup \{i_1,\cdots,i_{j-1}\}\setminus \{c_1,\cdots, c_{j-1}\})|T_{1,\cdots, w-1},i_{1,\cdots, j-1}]
$$
$$
\ge
{ \frac{1}{k}\left((1-\frac{\alpha}{k})f(S^*)-2f({S}_{1,\ldots, w-1} \cup \{i_1,\cdots,i_{j-1}\}\setminus \{c_1,\cdots, c_{j-1}\})\right)\ . }
$$  
}
%\end{align}
\end{lemma}
}

\mcomment{
\begin{proof}
In the algorithm~\ref{alg:main}, at the end of window $w$, we set %$S_{1,\cdots, w-1} = {S}_{1,\cdots, w-1} \setminus \bar{S}_w$.
%$S_{1,\cdots, w} = S_{1,\cdots, w-1}\cup S_w \setminus \bar{S}_w$.
$S_{1,\cdots, w} = \bar{S}_w$.
Suppose $a\in s_j\cap S^*$. 
Moreover, let $S'$ be the extension of $S(w-1,\tilde{\tau}_w,j-1)$ to a base of $\mathcal{M}$, and $\pi$ be the bijection from Brualdi lemma (refer to Lemma~\ref{lem:Brualdi}) from $S^*$ to $S'$.
Thus the expected value of the function $g$ on the element selected by the algorithm in slot $s_j$ (the element with maximum $g$ in the slot $s_j$) would be as follows. 
%\begin{eqnarray*}
\begin{align*}
&\Ex[f(S(w-1,\tilde{\tau}_w,j)|T, i_{1,\ldots, j-1}]  
\\ \ge& 
\Ex[f( (S(w-1,\tilde{\tau}_w,j-1)\cup\{a\})\setminus \{\pi(a)\}) 
 |T, i_{1,\ldots, j-1}, a\in S^*\cap Z_{s_j}] 
\\ \ge &
\Ex[f(S(w-1,\tilde{\tau}_w,j-1) \setminus \{\pi(a)\} )
|T, i_{1,\ldots, j-1}, a\in S^*\cap Z_{s_j}]+
\\ & \Ex[\Delta_f(a|S(w-1,\tilde{\tau}_w,j-1)\setminus \{\pi(a)\} )
|T, i_{1,\ldots, j-1}, a\in S^*\cap Z_{s_j}]
\\ \ge &
\Ex[f(S(w-1,\tilde{\tau}_w,j-1)\setminus \{\pi(a)\} )
|T, i_{1,\ldots, j-1}, a\in S^*\cap Z_{s_j}]
\\+&\Ex[\Delta_f(a|S(w-1,\tilde{\tau}_w,j-1) )
|T, i_{1,\ldots, j-1}, a\in S^*\cap Z_{s_j}].
\end{align*}
%\end{eqnarray*}
The first inequality is from the definition of function $g$ as it is defined in equation~\ref{eq:g}. The last inequality from submodularity of $f$.
Now from the last inequality  and lemma~\ref{replaced} we have
\begin{align*}
\Ex[f({S}(w-1,\tilde{\tau}_w,j)  |T, i_{1,\ldots, j-1})]\ge &
 (1-\frac{1}{k-\alpha} ) f(S(w-1,\tilde{\tau}_w,j-1) )\\
 &+ \Ex[ \Delta_f(a|{S}(w-1,\tilde{\tau}_w,j-1) \})
 |T_{1,\ldots, w-1}, i_{1,\ldots, j-1}, a\in S^*\cap Z_{s_j}]. 
\end{align*}
Now from lemma~\ref{lem:asGoodas} and the above inequality we can show
\begin{align*}
\Ex[f({S}(w-1,\tilde{\tau}_w,j)  |T, i_{1,\ldots, j-1})]&\ge
(1-\frac{1}{k-\alpha} ) f(S(w-1,\tilde{\tau}_w,j-1) )&\\
&+ \frac{1}{k} ((1-\frac{\alpha}{k})f(S^*)-f({S}(w-1,\tilde{\tau}_w,j-1)) )\ . 
\end{align*}
Thus,
\begin{align}  %\label{recursion}
\Ex[f({S}(w-1,\tilde{\tau}_w,j) ) 
- f(S(w-1,\tilde{\tau}_w,j-1) )] \nonumber 
\ge
 \frac{1}{k}((1-\frac{\alpha}{k})f(S^*)-2\rho f({S}(w-1,\tilde{\tau}_w,j-1))  \ . 
 %\label{recursion}
\end{align}
Hence,
\begin{align*}
&\Ex[g(i_j,S(w-1,\tilde{\tau}_w,j-1)) | T_{1,\cdots, w-1}, i_{1,\ldots, j-1}] \ge 
 %(1-\frac{1}{k-\alpha})
 \frac{1}{k}
 ((1-\frac{\alpha}{k})f(S^*)-2\rho f(S(w-1,\tilde{\tau}_w,j-1))).\
\end{align*}
\end{proof}
}

\mcomment{
%\subsection
\textbf{Proof of Lemma~\ref{cor:asGoodas}}
\begin{proof}
Let $\pi_0= (1-\frac{\alpha}{k}) f(S^*) - 2\rho\Ex[f(S_{1,\ldots, w-1}) | T_{1,\ldots, w-1}=T]$, and for $j \ge 1$,
\begin{align}
\pi_j:=(1-\frac{\alpha}{k}) f(S^*) - 2\rho\Ex[f(S(w-1,\tilde{\tau}_w,j)) | T_{1,\ldots, w-1}=T, i_1,\ldots, i_{j-1}],
\end{align}
Then, subtracting and adding $\frac{1}{2}(1-\frac{\alpha}{k}) f(S^*)$ from the left hand side of lemma~\ref{exg}, and taking expectation conditional on $T_{1,\ldots, w-1}=T, i_1, \ldots, i_{j-2}$, we get
\[-\frac{1}{2} ( \Ex[\pi_{j} | T, i_1, \ldots, i_{j-2}] + \pi_{j-1} ) \ge \frac{\rho}{k} \pi_{j-1}\]
which implies
\[\Ex[\pi_j|T, i_1, \ldots, i_{j-2}] \le \left(1-\frac{2\rho}{k}\right) \pi_{j-1} \le \left(1-\frac{2\rho}{k}\right)^j \pi_0\ .\]
By martingale stopping theorem, this implies:
\[\Ex[\pi_t|T] \le \Ex\left[\left(1-\frac{2\rho}{k}\right)^t \left| T\right. \right] \pi_0 \le \Ex\left[e^{-2t/(k-\alpha)}| T\right] \pi_0\ .\]
where stopping time $t=|\tilde{\tau}_w|\le \alpha \beta$ is bounded. 
Therefore, by martingale stopping theorem we can replace $t$ with $|\tilde{\tau}_w|$.
%($t=|\tilde \tau_w| \le \alpha\beta$ is bounded, therefore, martingale stopping theorem can be applied).
\end{proof}
}

\toRemove{
Next, we compare $\gamma(\tilde \tau_w)$ to $S_w=\gamma(\tau^*)$ . Here, $\tau^*$ was defined has the `best' greedy subsequence of length $\alpha$ (refer to \eqref{eq:Sw} and \eqref{eq:taustar}). To compare it with $\tilde \tau_w$, we need a bound on size of $\tilde \tau_w$. We use concentration inequalities proved in~\cite{us}:

\toRemove{
\begin{lemma}
\label{lem:lengthtau}
For any real $\delta\in (0,1)$, 
and if $k \ge \alpha\beta$, $\alpha \ge 8\log(\beta)$ and $\beta \ge 8$, 
%$\beta \ge \frac{3}{\delta}$, $\alpha \ge 4 \log(3\beta/\delta)$, and $\frac{2\alpha}{k} \le \frac{\delta}{3}$, 
then given any $T_{1,\ldots, w-1}=T$,
$$(1-\delta)\left(1-\frac{4}{\beta}\right)\alpha \le |\tilde \tau_w| \le (1+\delta)\alpha,$$
with probability $1-\exp(-\frac{\delta^2\alpha}{8\beta})$.
\end{lemma}
}
\toRemove{
\begin{proof}
By definition,
$$|\tilde \tau_w| = |s\in w: Z_s\ne \phi|\ .$$
Again, we use $s'\prec_w s$ to denote all slots before $s$ in window $w$. Then, from Lemma \ref{lem:Zs}, given $T_{1,\ldots, w-1}=T$, for all $i\cap S^*$ and slot $s$ in window $w$, $\Pr[i\in Z_s | Z_{s'}, s'\prec_w s, T]$ is either $0$ or $1/(k\beta)$. Therefore,
$$\Pr[Z_s \ne \phi | T, Z_{s'}, s'\prec_w s]\le \sum_{i\in S^*}  \frac{1}{k\beta} = \frac{1}{\beta}\ .$$
Therefore $X_s=|s'\preceq_w s: Z_{s'}\ne \phi| - \frac{s}{\beta}$ is a super-martingale, with $X_s-X_{s-1}\le 1$. Since there are $\alpha \beta$ slots in window $w$, $X_{\alpha\beta}=|s\in w: Z_{s}\ne \phi| - \alpha$.  Applying Azuma-Hoeffding inequality to  $X_{\alpha\beta}$ (refer to Lemma \ref{lem:azuma}) we get that 
\begin{equation}
\label{eq:upper}
\Pr\left( |s\in w: Z_s \ne \phi| \ge (1+\delta) \alpha |T\right) \le \exp\left(-\frac{\delta^2\alpha}{2\beta}\right)
\end{equation}
which proves the desired upper bound.

For lower bound, first observe that every $i\in S^*$ appears in $\cup_{s\in w} Z_s$ independently with probability $\frac{\alpha}{k}$. Using Chernoff bound for Bernoulli random variables (Lemma \ref{lem:Chernoff}),  for any $\delta\in(0,1)$
\begin{equation}
\label{eq:lower1}
\Pr(||\cup_{s\in w}Z_s| -\alpha| > \delta\alpha) \le \exp(-\delta^2\alpha/3) \ .
\end{equation}
%\begin{equation}
%\label{eq:lower15}
%\Pr\left(||S^* \cap Z_s| - \frac{1}{\beta}| \ge \frac{\delta}{\beta} |T\right) \le \exp(\frac{-\delta^2}{2k\beta^2})
%\end{equation}

Also, from independence of $i\in Z_s|T$ and  $i'\in Z_s|T$ for any $i,i'\in S^*, i\ne i'$ (refer to Lemma \ref{lem:Zs}),
$$\Pr(i,i'\in Z_s|T, i,i'\notin Z_{s'} \text{ for any } s'\prec_w s) \le  \frac{1}{k^2\beta^2}$$
for any $s\in w$; so that
\begin{equation}
\label{eq:lower10}
\Pr\left(|Z_s|=1|T,  Z_{s'}, s'\prec_w s\right) \ge  \frac{k-|Z_{s'}: s'\prec_w s|}{k\beta}-\frac{1}{\beta^2} \ge \left(1-\frac{2\alpha}{k} \right)\frac{1}{\beta} - \frac{1}{\beta^2}- e^{-\frac{\alpha}{4}} =:p \ .
\end{equation}
where in the last inequality we substituted the upper bound  on $ |Z_{s'}: s'\prec_w s|$ from \eqref{eq:lower1}. 
Specifically, using  \eqref{eq:lower1} with $\delta=3/4$, we obtained  that $|Z_{s'}: s'\prec_w s|\le (1+\frac{3}{4})\alpha \le 2\alpha$ with probability $\exp(-\alpha/4)$. 
%Then, substituing 
%$$\Pr(|Z_s|>1|T, i,i'\notin Z_{s'} \text{ for any } s'\prec_w s) \le  \frac{1}{\beta^2}$$
%Also if  $\beta\ge \frac{3}{\delta'}$, $\alpha \ge  4 \log(3\beta/\delta')$, and $\frac{2\alpha}{k}\le \frac{\delta'}{3}$,  we have $ p :=\left(1-\frac{2\alpha}{k} - \frac{1}{\beta}\right)\frac{1}{\beta} - e^{-\frac{\alpha}{4}} \ge  (1-\delta')\frac{1}{\beta}$.
Also if $\alpha \ge  8 \log(\beta)$, and $k\ge \alpha\beta$,  we have $ p :=\left(1-\frac{2\alpha}{k} - \frac{1}{\beta}\right)\frac{1}{\beta} - e^{-\frac{\alpha}{4}} \ge  (1-\frac{4}{\beta})\frac{1}{\beta}$.

Now, applying Azuma-Hoeffding inequality (Lemma \ref{lem:azuma}), the total number of slots (out of $\alpha\beta$ slots) for which $|Z_s|=1$ can be lower bounded by:

 %we can bound the probability of another item from $S^*$ appearing in the same slot as item $i$. %
%That is, for any $i\in S^*$, %in $Z_s$ for some slot $s$: 
%$$\Pr(Y_i\in w, |Z_{Y_i}|>1, |T) \le \sum_{s\in w} \sum_{i'\in S^*, i'\ne i} \Pr(i,i'\in Z_s| T) = k \alpha\beta\frac{1}{(k\beta)^2} \le \frac{\alpha}{k\beta}$$
%$$\Pr(i: |Z_s|>1 for Y_i=s) \le \alpha\beta \frac{1}{(k\beta)^2} = \frac{\alpha}{k^2\beta}$$
%of these items appearing together in $S^*$, to get
%$$\Pr[i,i'\in Z_s] \le \sum_{i\in S^*, i'\in S^*}  \frac{1}{(k\beta)^2} = \frac{1}{\beta^2}$$

%$$\Pr[|Z_s|>1 | T, Z_{s'}, s'\prec_w s]\le \sum_{i\in S^*, i'\in S^*}  \frac{1}{(k\beta)^2} = \frac{1}{\beta^2}$$

%Therefore, Chernoff bound, 
%applying Azuma-Hoeffding inequality (for super-martingales), 
%the total number of items from $S^*$ who are not alone in their slots in $w$ can be bounded by:
\begin{equation}
\label{eq:lower2}
%\Pr(|\{i: Y_i\in w \text{ and } |Z_{Y_i}|>1\}| \le (1-\delta) \frac{\alpha}{\beta}) \le \exp(-\frac{\delta^2\alpha}{2\beta})
\Pr\left(|\{s \in w:|Z_s|=1\}| \le (1-\delta)p\alpha\beta|T\right) \le \exp\left(-\frac{\delta^2 p^2 \alpha \beta}{2}\right) \ .
\end{equation}
 Substituting $p\ge  (1-\frac{4}{\beta})\frac{1}{\beta}$,
$$\Pr\left(|\{s \in w:|Z_s|=1\}| \le (1-\delta)(1-\frac{4}{\beta})\alpha|T\right) \le \exp\left(-\frac{\delta^2 (1-4/\beta)^2 \alpha}{2\beta}\right)\ . $$
We further substitute $\beta \ge 8$ in the right hand side of the above inequality, to bound the probability by $\exp(-\delta^2\alpha/8\beta)$.
%$$\Pr(|\{s \in w:|Z_s|=1\}| \ge (1-\delta)(1-\delta')\alpha|T) \le \exp(-\frac{\delta^2 (1-\delta')^2 \alpha}{2\beta})$$
%The desired lower bound on $\tilde \tau_w$ is then obtained by using $\delta'=\delta$.
%$$\Pr[|Z_s|\ge 1 | T, Z_{s'}, s'<s, s'\in w]\ge \sum_{i\in S^*\cup_{s'<s} Z_s'}  \frac{1}{k\beta} = \frac{k-|\cup_{s'<s} Z_s'|}{k\beta} =:x_s$$

%Since $k\ge \alpha\beta$, 
%Using \eqref{eq:lower1} and \eqref{eq:lower2}, and taking union bound, we have that for any $\delta\in(0,1)$, with probability at least $1-\exp(\frac{-\delta^2 \alpha}{2}) - \exp(\frac{-\delta^2\alpha}{\beta^3})$, at least $(1-\delta)\alpha$ items from $S^*$ are part of $\cup_{s\in w} Z_s$,  and further at most  $(1-\delta)\frac{\alpha}{\beta}$ slots contain multiple of these items. Therefore, $Z_s$ must be non-empty in at least $\left(1-\frac{1}{\beta}\right)(1-\delta)\alpha$ slots. This proves the required lower bound

%\scomment{using deviation bounds as in the earlier proofs}
\end{proof}
}

\begin{lemma}
%[Corollary of Lemma \ref{lem:lengthtau}]
[proved in~\cite{us}]
\label{cor:lengthtau}
For any real $\delta'\in (0,1)$,  if parameters $k,\alpha, \beta$ satisfy \settinga, then given any $T_{1,\ldots, w-1}=T$, with probability at least $1-\delta' e^{-\alpha/k}$,
$$|\tilde \tau_w| \ge (1-\delta') \alpha\ . $$
\end{lemma}
}

\toRemove{
\begin{proof}
We use the previous lemma with $\delta=\delta'/2$ to get lower bound of $(1-\delta')\alpha$ with probability $1-\exp(-(\delta')^2\alpha/32\beta)$. Then, substituting 
%$\alpha \ge 8\beta^2$,
$ k\ge \alpha\beta \ge \frac{64\beta}{(\delta')^2} \log(1/\delta')$ so that using $\beta \le \frac{k(\delta')^2}{64 \log(1/\delta')}$ we can bound the violation probability by
$$\exp(-(\delta')^2 \alpha/32\beta)\le \exp(-(\delta')^2 \alpha/64\beta)\exp(-\alpha/k) \le \delta' e^{-\alpha/k}.$$
where the last inequality uses $\alpha\ge 8\beta^2 \log(1/\delta')$ and $\beta \ge 8/(\delta')^2$.
%$\delta :=\frac{\log(1-\delta')}{2\alpha}$. Note that $\delta \ge \frac{\delta'}{2\alpha}$. 
\end{proof}
}

\mcomment{
\subsection{Proof of Lemma~\ref{lem:Sw}}
\begin{lemma}
\label{lem:Sw}
For any real $\delta'\in (0,1)$, if parameters 
$k,\alpha, \beta$ satisfy \settinga, then
\[\Ex\left[(1-\frac{\alpha}{k}) \OPT -2\rho f(S_{1,\ldots, w})|T_{1,\ldots, w-1}\right] \le 
(1-\delta') e^{-2\alpha/(k-\alpha)} \left((1-\frac{\alpha}{k}) \OPT - 2\rho f(S_{1,\ldots, w-1})\right)\ .\]
\end{lemma}
\begin{proof}
The lemma follows from substituting %Lemma \ref{cor:lengthtau} 
Lemma 14 of~\cite{us}
in Lemma \ref{cor:asGoodas}.
%Using previous lemma with $\delta:=\delta'/2$ we get $|\tilde \tau_w|\ge (1-\delta')\alpha$ with probability at least $1-\delta'$. Therefore, we can derive
%Since $e^{-t/k}$ is a convex decreasing function in $t$,
%$$\Ex[e^{-|\tilde \tau_w|/k} |T ] \le (1-\frac{}{})e^{-(1-\delta')\alpha/k}$$
\end{proof}
}

\toRemove{
\begin{proof}
The lemma follows from substituting %Lemma \ref{cor:lengthtau} 
Lemma 15 of~\cite{us}
in Lemma \ref{cor:asGoodas}.
Using previous lemma with $\delta:=\delta'/2$ we get $|\tilde \tau_w|\ge (1-\delta')\alpha$ with probability at least $1-\delta'$. Therefore, we can derive
Since $e^{-t/k}$ is a convex decreasing function in $t$,
$$\Ex[e^{-|\tilde \tau_w|/k} |T ] \le (1-\frac{}{})e^{-(1-\delta')\alpha/k}$$
\end{proof}

\begin{proof}
We use the previous lemma with $\delta=\delta'/2$ to get lower bound of $(1-\delta')\alpha$ with probability $1-\exp(-(\delta')^2\alpha/32\beta)$. Then, substituting 
%$\alpha \ge 8\beta^2$,
$ k\ge \alpha\beta \ge \frac{64\beta}{(\delta')^2} \log(1/\delta')$ so that using $\beta \le \frac{k(\delta')^2}{64 \log(1/\delta')}$ we can bound the violation probability by
$$\exp(-(\delta')^2 \alpha/32\beta)\le \exp(-(\delta')^2 \alpha/64\beta)\exp(-\alpha/k) \le \delta' e^{-\alpha/k}.$$
where the last inequality uses $\alpha\ge 8\beta^2 \log(1/\delta')$ and $\beta \ge 8/(\delta')^2$.
%$\delta :=\frac{\log(1-\delta')}{2\alpha}$. Note that $\delta \ge \frac{\delta'}{2\alpha}$. 
\end{proof}

}

\subsection{Proof of Proposition~\ref{opttheoremMatroid}}

\toRemove{
\begin{lemma}
\label{lem:Sw}
%For any $\delta'\in (0,1)$,  if parameters $k, \alpha\ge 1, \beta\ge 1$ are such that 
%$\alpha \ge 4 \log(36\alpha^2/\delta'^2)$, $\beta \ge 6\alpha/\delta'$, and $k\ge 12\alpha^2/\delta'$, then
For any real $\delta'\in (0,1)$, if parameters 
$k,\alpha, \beta$ satisfy \settinga, then
%\mbox{$k \ge \alpha\beta$}, \mbox{$\beta\ge \frac{8}{(\delta')^2}$}, $\alpha\ge 8\beta^2 \log(1/\delta')$, then %probability at least $1-\delta'$,
$$\Ex\left[\frac{k-\alpha}{k} \OPT -2f(S_{1,\ldots, w})|T_{1,\ldots, w-1}\right] \le (1-\delta') e^{-2\alpha/k} \left(\frac{k-\alpha}{k} \OPT - 2f(S_{1,\ldots, w-1})\right)\ .$$
\end{lemma}
\begin{proof}
The lemma follows from substituting Lemma \ref{cor:lengthtau} in Lemma \ref{cor:asGoodas}.
%Using previous lemma with $\delta:=\delta'/2$ we get $|\tilde \tau_w|\ge (1-\delta')\alpha$ with probability at least $1-\delta'$. Therefore, we can derive
%Since $e^{-t/k}$ is a convex decreasing function in $t$,
%$$\Ex[e^{-|\tilde \tau_w|/k} |T ] \le (1-\frac{}{})e^{-(1-\delta')\alpha/k}$$
\end{proof}
}

%\matroidThm

\toRemove{
\begin{theorem} \label{opttheorem}
(theorem 1 in the paper) For any constant $\epsilon>0$, there exists an online algorithm (Algorithm \ref{alg:main}) for the \nameOfProblemMatroidSL\ that achieves a competitive ratio of $\frac{1}{2}(1-\frac{1}{e^2} -\epsilon -O(\frac{1}{k}))$, with shortlist of size $\eta_\epsilon(k)=O(k)$. Here,  $\eta_\epsilon(k)=O(2^{poly(1/\epsilon)}k)$. The running time of this online algorithm is $O(nk)$.
\end{theorem}
}

\begin{proof}
Now from Lemma~\ref{lem:Sw}, we have,
%\begin{prop}
%\label{prop:first}
for any real $\delta'\in (0,1)$, if parameters 
$k,\alpha, \beta$ satisfy \settinga, then the set $S_{1,\ldots, W}$ tracked by Algorithm \ref{alg:card} satisfies

\begin{align*}
\mathbb{E}[f(S_{1,\ldots, W})] &\ge   (1-\delta') (\frac{1}{2}(1-1/e^{2}) ) \OPT 
%\\ &\ge (1-\frac{\alpha}{k}) (1-\delta')^2 (\frac{1}{2}(1-1/e^{2}) ) \OPT 
%\\ & \ge (1-\delta')^3 (\frac{1}{2}(1-1/e^{2}) ) \OPT
\end{align*}
%\end{prop}
%By setting $\delta'=\epsilon/4$, 

\toRemove{
\begin{proof}
By multiplying the inequality Lemma \ref{lem:Sw} from $w=1, \ldots, W$, where $W=k/\alpha$, we get 
$$\mathbb{E}[f(S_{1,\ldots, W})] \ge (1-\delta')(\frac{1}{2}(1-1/e^2)) (1-\frac{\alpha}{k}) \OPT.$$
Then, using $1-\frac{\alpha}{k}\ge 1-\delta'$ because $k\ge \alpha \beta \ge \frac{\alpha}{\delta'}$, we obtain the desired statement.
\end{proof}
}
%\begin{lemma}
%$$\Ex[f(S_{1,\ldots, w-1} \cup_{s\in w} Z_s) - f(S_{1,\ldots,w-1})|T_{1,\ldots, w-1} =T] \ge \frac{\alpha}{k}\Ex[f(S^*)-f(S_{1,\ldots, w-1})|T_{1,\ldots, w-1} =T]$$
%\end{lemma}

%------------------

%\scomment{End:Trying out something------------------------} 

Now, we compare $f(S_{1\ldots, W})$ to $f(S\cap R)$, %where $A^*=S_{1\ldots, W} \cap A$, 
with $R$ being the shortlist returned by Algorithm \ref{alg:matroid}. The main difference between the two sets is that in the construction of shortlist $R$, Algorithm \ref{alg:matroidmax} is being used to compute the argmax in the definition of $H_{\ell}$, in an online manner. This argmax may not be computed exactly, so that some items from $S_{1\ldots, W}$ may not be part of the shortlist $R$. 

\toRemove{
We use the following guarantee for Algorithm~\ref{alg:matroidmax} to bound the probability of this event.
}

%\begin{prop}
%\label{maxanalysis}
%Algorithm~\ref{alg:SIIImax}, with parameter $u=n\epsilon/2$,  and shortlist of size $L= (2+\sqrt{3})\ln(2/\epsilon)$ selects the maximum element with probability $(1-\epsilon)$, \end{prop}

%\scomment{I thought I changed the statement of the above proposition, did you change it back? Algorithm~\ref{alg:SIIImax}  only takes inputs $N, \delta$, the setting of $u, L$ is fixed in Algorithm~\ref{alg:SIIImax}  so it should not be mentioned in the proposition, replace the following:
%}
%\mcomment{No I just changed the format of inequality from $1-\epsilon-\delta$ to $1-\epsilon$}

\toRemove{
\begin{restatable}{prop}{maxanalysis}
\label{maxanalysis}
For any $\delta\in (0,1)$, and input $I=(a_1,\ldots, a_N)$, Algorithm~\ref{alg:matroidmax}
returns $A^*:= \max_{i\in A} g(a_i,S)$ with 
probability $(1-\delta)$. 
\end{restatable}

The proof is similar to Proposition 3 in~\cite{us}.
}
%\scomment{where is the proof of this? add intuition and reference to proof}
%The proof of the above proposition appears in Appendix \ref{app:msubm}. Intuitively, it follows from the observation that if we select every item that improves the maximum of items seen so far, we would have selected $\log(N)$ items in expectation. The exact proof involves showing that on waiting $n\delta/2$ steps and then selecting maximum of every item that improves the maximum of items seen so far, we miss the maximum item with at most $\delta$ probability, and select at most $O(\log(1/\delta))$ items with probability $1-\delta$.
%\scomment{Removed:We prove a more general theorem in the Appendix (Theorem~\ref{hprob}).}
%\scomment{There are some todos with respect to this proof. Please check the comments in appendix.}

Similar to Lemma 16 in~\cite{us}, we can show that each element in $R$ gets selected by the algorithm with probability at least $1-\delta$. More precisely,
%\begin{lemma}
%\label{online}
let $A$ be the shortlist returned by Algorithm \ref{alg:card}, and $\epsilon$ is the parameter used to call Algorithm \ref{alg:matroid}. Then, for given configuration $Y$, for any item $a$, we have \[Pr(a\in A|Y, a\in SH(w,\ell,s) \ge 1-\epsilon/2\ .\]
%\end{lemma}

\toRemove{
\begin{proof}
From Lemma~\ref{config} by conditioning on $Y$, the set $S_{1,\cdots, W}$ is determined. Now if $a\in S_{1,\dots, w}$, 
%$a=argmax \gamma(\tau)$
then for some slot $s_j$ in an $\alpha$ length subsequence $\tau$ of some window $w$, we must have 
%$$a = \arg \max_{i\in s_j \cup R_{1, \ldots, w-1}} f(S_{1, \ldots,w-1} \cup \gamma(\tau) \cup \{i\}) - f(S_{1, \ldots, w-1} \cup \gamma(\tau)).$$
$$a = \arg \max_{i\in s_j \cup R_{1, \ldots, w-1}} g(i,S_{1, \ldots,w-1} \cup \gamma(\tau) \setminus \zeta(\tau)).$$ 

Note that in contrast with the algorithm for cardinality constraints, now one element can be removed from $S_{1,\cdots, w-1}$
and added back in the next windows. 
Let $w'$ be the first window that $a$ has been added to $S_{1,\cdots, w'}$ and has not been removed later on in the next windows $w',\cdots, w$.
%Let $w'$ be the first such window, 
Also let $\tau', s_{j'}$ be the corresponding subsequence and slot. Then, it must be true that 
%$$a = \arg \max_{i\in s_{j'}} f(S_{1, \ldots,w'-1} \cup \gamma(\tau') \cup \{i\}) - f(S_{1, \ldots, w'-1} \cup \gamma(\tau')).$$
$$a = \arg \max_{i\in s_{j'}} g(i,S_{1, \ldots,w'-1} \cup \gamma(\tau')\setminus \zeta(\tau') ).$$ 
(Note that the argmax in above is not defined on $R_{1,\cdots, w'-1}$).
The configuration $Y$ only determines the set of items in the items in slot $s_{j'}$, the items in $s_{j'}$ are still randomly ordered (refer to Lemma \ref{config}). Therefore, from Proposition~\ref{maxanalysis}, with probability $1-\delta$, $a$ will be added to the shortlist $A_{j'}(\tau')$ by Algorithm~\ref{alg:matroidmax}. Thus $a\in A \supseteq A_{j'}(\tau')$ with probability at least $1-\delta$.
\toRemove{If $a\in R_{1,\cdots, w-1}$ then $a$ has appeared in a window before $w$ for the first time, say $w'$. Since $a\in R_{1,\cdots, w-1}$ there is $\tau'$, such that
$a := \arg \max_{i\in s_{\ell}} f(S_{1, \ldots,w'-1} \cup \gamma(\tau') \cup \{i\}) - f(S_{1, \ldots, w'-1} \cup \gamma(\tau'))$ 
(Note that the argmax in above is not defined on $R_{1,\cdots, w'-1}$).
The configuration $Y$ only determines the set of items in the items in slot $s_{j'}$, the items in $s_{j'}$ are still randomly ordered (refer to Lemma \ref{..}).
The permutation of elements in $s_{\ell}$ defines whether or not the online Algorithm~\ref{alg:SIIImax} selects $a$ or not. 
Therefore, from Theorem~\ref{maxanalysis}, with probability $1-\delta$, $a$ will be added to the shortlist $A_{j'}(\tau')$ by Algorithm~\ref{alg:matroidmax}. Thus $a\in A \supseteq A_{j'}(\tau')$ with probability at least $1-\delta$.
Thus $a\in H_{1,\cdots, w'-1}$ with probability at least $1-\delta$.
Now If $a \notin R_{1,\cdots, w-1}$ and $a\in s_j$, then the permutation of elements in $s_{j}$ defines whether or not the online Algorithm~\ref{alg:matroidmax} selects $a$ or not.
Therefore again from theorem~\ref{maxanalysis}, 
$a\in H_{1,\cdots, w'-1}$ with probability at least  $1-\delta$.}
\end{proof}
}
Therefore using Lemma~\ref{sample},
%\begin{prop}
\label{prop:online}
\[\Ex[f(S\cap R)] \ge (1-\frac{\epsilon}{2})\mathbb{E}[f(S_{1,\cdots, W})].\]
%where $A^*:= S_{1,\cdots, W} \cap A$ is the %size $k$ 
subset of shortlist $A$ returned by Algorithm \ref{alg:card}.
%\end{prop}
%\begin{proof}
%The proof is similar to the proof in~\cite{us}.
%\end{proof}
Thus by setting $\delta'=\epsilon/4$, for $k>\alpha \beta$, we obtain lower bound $\frac{1}{2}(1-1/e^2-\epsilon)OPT$.
The running time of the algorithm is discussed in the streaming section.

\end{proof}
%%%%%%%%%%%%%%%%%%%%%%%%%%

%\subsection{Bounding $\Ex[f(A^*)]/\OPT$}

\mcomment{
\subsection{Missing Proof for the Preemption model and 
Shortlist of size at most $k$ (Theorem 2)}
}

\toRemove{
Finally we focus on the special case where the size of shortlist is at most $k$. We can get a constant competitive algorithm even with the slight relaxation of the \textit{matroid secretary problem} 
to the case that we allow the algorithm to select a shortlist of size at most $k=rk(\mathcal{M})$. 
The algorithm finally outputs an independent subset of this shortlist of size $k$. There was no constant compettetive algorithm even for this natural relaxation of \textit{matroid secretary problem}.
Also we are not aware of any direct way to prove a constant factor guarantee for this simple relaxation without using the techniques that we develop using $(\alpha,\beta)$-windows. 
}

%The Algorithm~\ref{alg:main}s becomes very simple in this case:

\toRemove{
\begin{algorithm*}[h!]
  %\caption{~\bf{Select-If-it-Improves}($I , u$)}
  \caption{~\bf{Algorithm for {\bf submodular} matroid secretary with shortlist of size $k$}}
  \label{alg:simple} 
\begin{algorithmic}[1]
\State Inputs: number of items $n$, submodular function $f$, parameter $\epsilon \in (0,1]$. 
\State Initialize: $S_0 \leftarrow \emptyset, R_0 \leftarrow \emptyset, A \leftarrow \emptyset, A^* \leftarrow \emptyset$, constants $\alpha \ge 1, \beta \ge 1$ which depend on the constant $\epsilon$.
\State Divide indices $\{1,\ldots, n\}$ into $(\alpha, \beta)$ windows. %as prescribed by Definition \ref{def:windows}.
%Divide the sequence of candidates into consecutive groups of $\frac{n}{\beta k}$ candidates, referred to as slots (or buckets). And, divide the sequence of slots into consecutive groups of $\alpha \beta$ slots, referred to as {\it windows}.
%===========================
\For {window $w= 1, \ldots, k/\alpha$} 
%\State For every $\alpha$-length subsequence $\tau=(s_1,\ldots, s_\alpha) \subseteq [\alpha\beta]$ of slots in window $w$, define 
%$$\gamma(\tau):=\{i_1, \ldots, i_\alpha\}$$
%where 
%$$i_j := \arg \max_{i\in V_{s_j,w} \cup R_{1,\ldots, w-1}} f(S_{1,\ldots,w-1} \cup \{i_1\ldots, i_{j-1}\} \cup \{i\}) - f(S_{1,\ldots,w-1} \cup \{i_1\ldots, i_{j-1}\})$$
%\State Define $R_w:=\{\cup_{\tau} \gamma(\tau)\}.$ 

%\State Process the online inputs in window $w$ using the subroutine in Algorithm \ref{alg:tmpWindow} to select a subset $H_w$ of items. 
 \For {every slot $s_j$ in window $w$, $j=1,\ldots, \alpha\beta$}
  \State Concurrently for all subsequences of previous slots $\tau\subseteq \{s_1, \ldots, s_{j-1}\}$ of length $|\tau|<\alpha$ \label{li:subb}\\
  \hspace{0.44in} in window $w$, call the online algorithm in Algorithm \ref{alg:matroidmax} with the following inputs: 
  %\begin{center}
  \begin{itemize}%[leftmargin=0.7in]
  \item   number of items $N=|s_j|+1$, $\delta=\frac{\epsilon}{2}$, and
%  \scomment{You have to use $\delta$ smaller than $\epsilon$ to get $1-\frac{1}{e}-\epsilon$ in the final result.}
  \item item values $I=(a_0, a_1, \ldots, a_{N-1})$, with 
   
     \begin{eqnarray*} 
  a_0 & := & \max_{x\in R_{1,\ldots, w-1}} \Delta(x|S_{1,\ldots,w-1} \cup \gamma(\tau)\setminus \zeta(\tau)) \\
  %\max_{x\in R_{1,\ldots, w-1}} f(S_{1,\ldots,w-1} \cup \gamma(\tau) \cup \{x\}) - f(S_{1,\ldots,w-1} \cup \gamma(\tau)\}$
     a_\ell & := & \Delta(s_j(\ell)| S_{1,\ldots,w-1} \cup \gamma(\tau)\setminus \zeta(\tau) ),  \forall 0<\ell\le N-1
     \end{eqnarray*}
    %f(S_{1,\ldots,w-1} \cup \gamma(\tau) \cup \{i\}) - f(S_{1,\ldots,w-1} \cup \gamma(\tau)\})$
 where $s_j(\ell)$ denotes the $\ell^{th}$ item in the slot $s_j$. 
% \item $\delta = \frac{\epsilon}{{\alpha \beta \choose \alpha}}$.
  \end{itemize}
   %\end{center}
   %\mcomment{why do you divide by... the erros do not add up}  \scomment{Please add the required theorem showing this}  \mcomment{added lemma~\ref{online}}
\State Let $A_{j}(\tau)$ be the shortlist returned by  Algorithm \ref{alg:matroidmax} for slot $j$ and subsequence $\tau$. Add \\
\hspace{0.44in} all items except the dummy item $0$ to the shortlist $A$. %$H_w$, i.e, for all $\tau$,
 % $$H_w \leftarrow H_w\cup (A_{j}(\tau) \cap s_j)$$
 That is, \label{li:sube}
 $$A\leftarrow A\cup  (A(j)\cap s_j)$$
 \EndFor
%\State return $H_w$
% \State $A\leftarrow A\cup H_w$
 \State After seeing all items in window $w$, compute $R_w, S_w$ as before %defined in \eqref{eq:Rw} and \eqref{eq:Sw} respectively.
 \State $S_{1,\cdots, w} \leftarrow S_{1,\cdots, w-1}\cup S_w \setminus \bar{S}_w$
 \State $A^* \leftarrow A^*\cup (S_w \cap A)\setminus \hat{S}_w$
\EndFor
\State return $A$, $A^*$. %$A=T_1 \cup \cdots  \cup T_{W}$
\end{algorithmic}
\end{algorithm*}
}

%If the size of shortlist is exactly $k$ we get the following.

%\preemption

%\thmpreemption
\toRemove{
\begin{theorem} \label{thm:preemption}
For the matroid secretary problem in the preemption model, and matroid secretary problem 
that uses shortlist of size at most $\eta(k)=k$,
there is an algorithm 
%the algorithm~\ref{alg:main} 
%(with $\alpha=\beta=1$) 
that achieves a constant competitive ratio. %$\frac{1}{2} (1-1/e) (1-1/e^2-\epsilon)$.
\end{theorem}
}

\mcomment{
%\subsection{Preemption model and  Shorlitst of size at most $k$}
Finally we focus on the special case where the size of shortlist is at most $k$. We can get a constant competitive algorithm even with the slight relaxation of the \textit{matroid secretary problem} 
to the case that we allow the algorithm to select a shortlist of size at most $k=rk(\mathcal{M})$. 
The algorithm finally outputs an independent subset of this shortlist of size $k$. There was no constant compettetive algorithm even for this natural relaxation of \textit{matroid secretary problem}.
Also we are not aware of any direct way to prove a constant factor guarantee for this simple relaxation without using the techniques that we develop using $(\alpha,\beta)$-windows. 
\thmpreemption
\begin{proof}
We show that  algorithm~\ref{alg:main} 
with parameter $\alpha=\beta=1$ satisfies the above mentioned properties. Firstly,  algorithm~\ref{alg:main} (with $\alpha=1$, and $\beta=1$) uses shortlist of size $\eta(k)\le k$.
The reason is that the algorithm divides the input into exactly $k$ slots.
Also each window contains exactly one slot. 
The function $\gamma$ tries all $\alpha$-subsequences of a window which is exactly one slot. Thus $\gamma$ returns one element in that slot with hight value of $g(e,S)$ as defined in~\ref{eq:g}, which might cause removal of at most one element $\theta(S,e)$ from the current solution $S$. Therefore the algorithm has shortlist size at most $k$ and also satisfies the preemption model. Now by setting $\alpha=1, \beta=1$ we can get a constant compettetive ratio that  the error rate comes from lemma~\ref{lem:Sw}.
\toRemove{
Given that $|OPT|\le k$, we can extend the size of $OPT$ to a set of size exactly $k$, by adding some dummy elements.
Let's call that set $OPT'$.
In order to calculate the competitive ratio, we first compute the probability that one slot contains an element of optimal solution $OPT'$, i.e., the probability that $s\cap OPT'\neq \emptyset$, for a slot $s$ in window $w$. Since all $k$ elements of $OPT'$ are uniformly distributed, 
$$
Pr[s\cap OPT' \neq \emptyset | T_{1,\cdots, w-1} ] \ge 1- (1-1/k)^k.
$$
Therefore in lemma~\ref{cor:lengthtau}, $|\bar{\tau}_{w}|\ge 1$ with probability $1-1/e$. Hence 
$\mathbb{E}[f(S_{1,\ldots, W})] \ge \frac{1}{2}(1-1/e) (1-1/e^2)  \OPT.$
Thus by Lemma~\ref{cor:lengthtau} and~\ref{lem:Sw}, 
$$\mathbb{E}[f(A^*)] \ge  \frac{1}{2} (1-\epsilon)(1-1/e) (1-1/e^2)  \OPT.$$
}
\end{proof}
}
